# Supplementary material for: Dual Mesh Convolutional Networks for Human Shape Correspondence
Source: arXiv:2103.12459 source file (2021-10-16)
Supplement: Supplementary file 1 [file appendix.tex]

%\clearpage % or \cleardoublepage
%\addappheadtotoc
%\appendixpage

\section{Runtime and parameter count of network architectures}
\label{sec:network_details}

We report   the average execution time of a forward pass for a mesh of the re-meshed FAUST dataset for the different models  used in our experiments on a Tesla P100 GPU in \tab{remeshed_time}, as well as the number of parameters of these models.
All  methods have a similar number of parameters  and execution time, except SplineCNN which takes roughly twice longer to complete a forwards pass.
Note that for MoNet, the forwards pass time does not include the computation of the SHOT descriptors. \jakob{[Add how much time SHOT takes]}
SplineCNN also has roughy twice as many parameters as the other methods.
%which results from approximating 3-degree B-Spline over the mesh.
%\jakob{[I don't see how this doubles the nr of parameters. Nitika: can you explain more clearly?]}

\nitika{ Parameters - }

FeaStNet - 8X params

SplineConv - 125X params

Lin - Y params

Final FeaStNet Params - 8X + Y

Final SplineConv Params - 125X + Y

%SplineCNN - We report results using the architecture mentioned in \ssect{archi} in order to maintain uniformity across all experiments. 

%However, while trying to replicate the results using the original architecture $(99.2\%)$, we encounter exploding gradients. We add gradient clipping to keep the gradient norm under a certain threshold and obtain $97.3\%$ accuracy. \url{https://github.com/rusty1s/pytorch_geometric/issues/791/}

\begin{table}[h]
\begin{center}
    \begin{tabular}{llcc}
        \toprule
        Mesh Domain & Method & Time (in ms) & \#Params \\
        \midrule
        \multirow{3}{*}{Primal} & MoNet & $8.9 \pm 0.25$ & 1.4M \\
         & SplineCNN & $17.8 \pm 0.15$ & 3.1M \\
         & FeaStNet & $10.6 \pm 0.17$ & 1.4M \\
        \midrule
        \multirow{3}{*}{Dual} & FeaStConv--Dual & $10.4 \pm 0.14$ & 1.4M \\
         & DualConvMax & $8.6 \pm 0.57$ & 1.3M \\
         & DualConvInv & $9.4 \pm 0.16$ & 1.3M \\
        \bottomrule
    \end{tabular}
    \caption{Comparison of the number of parameters and average execution time of the forward-pass per mesh for re-meshed FAUST dataset.
%    \jakob{[Why do we have comparison of accuries here using different features? Can't we just drop the accuracies here? I guess the choice of feature has negligible impact on execution time?]}
    }
    \label{tab:remeshed_time}
\end{center}
\end{table}

%%%%%%%%%%%%%%%%%%%%%%%%%%%%%%%%

% \section{Additional Figures}
% \label{sec:additional_figs}

\begin{figure*}
	\setlength{\tabcolsep}{4.5pt}
	\resizebox{\textwidth}{!}{
	\scriptsize
	\begin{tabular}{lc|ccc|cc|cc}
	 & \textbf{Faust-Synthetic} & \textbf{MoNet} & \textbf{SplineCNN} & \textbf{FeaStNet} & \multicolumn{2}{c|}{\textbf{FeaStNet--Dual}} & \multicolumn{2}{c}{\textbf{DualConvMax}}
	\\
	 & \textbf{Reference} & \scriptsize{(SHOT)} & \scriptsize{(XYZ)} & \scriptsize{(XYZ)} & \scriptsize{(XYZ)} & \scriptsize{(XYZ+Normal)} & \scriptsize{(XYZ)} & \scriptsize{(XYZ+Normal)}
	 \\
	{\rotatebox{90}{\tiny{$0\%$}}} &
	\includegraphics[scale=0.042]{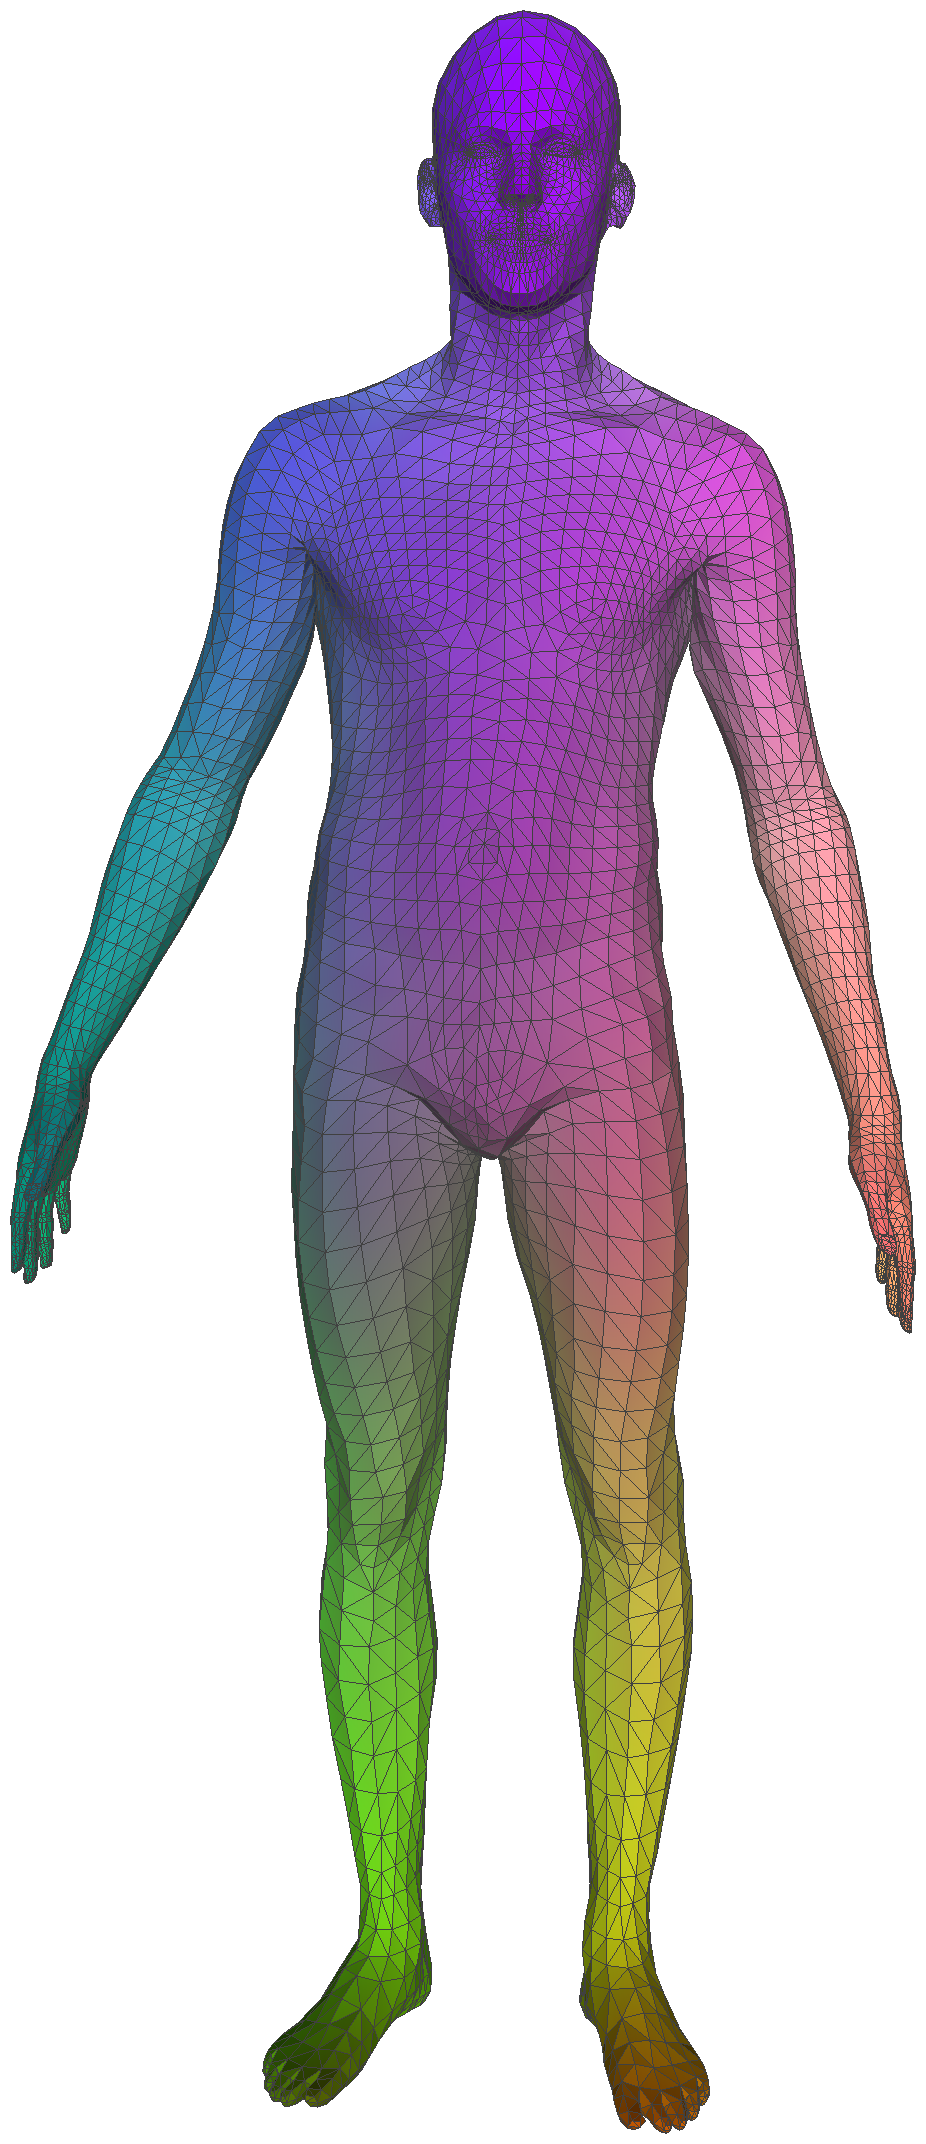} &
	\includegraphics[scale=0.054]{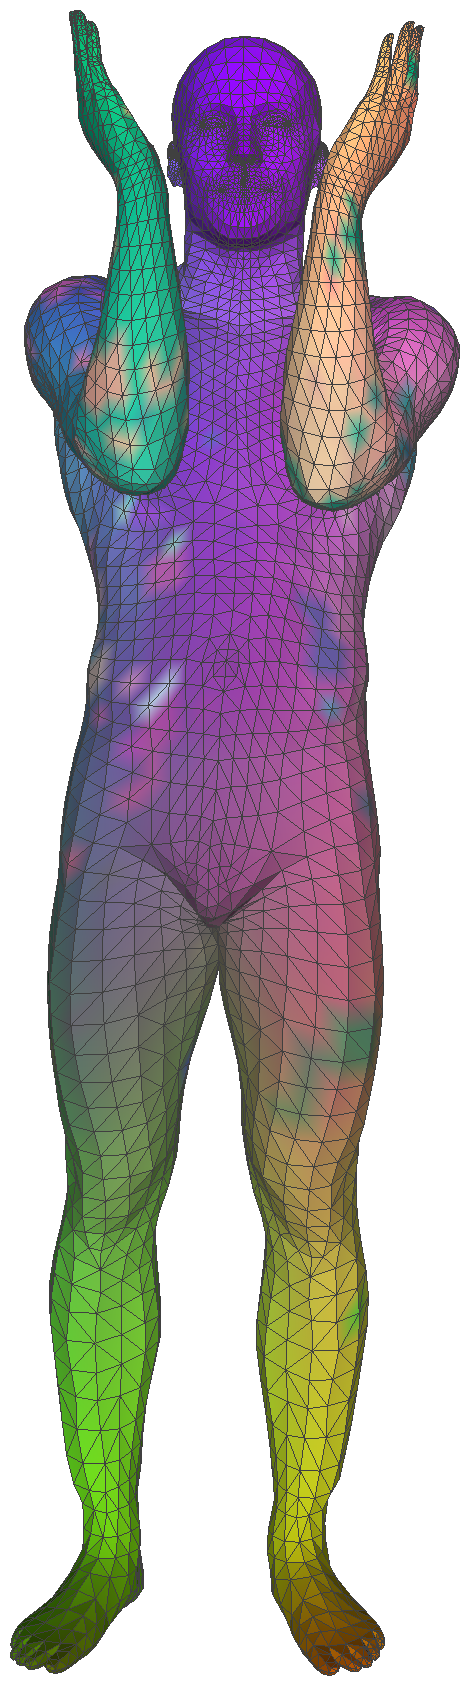} &
	\includegraphics[scale=0.054]{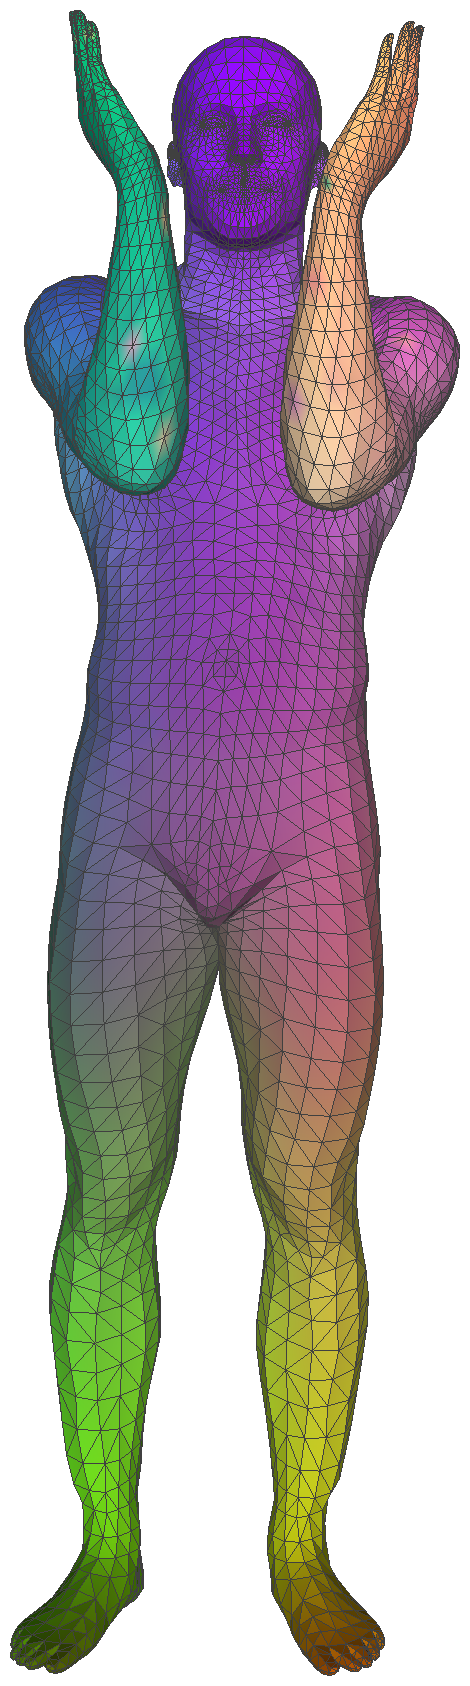} &
	\includegraphics[scale=0.061]{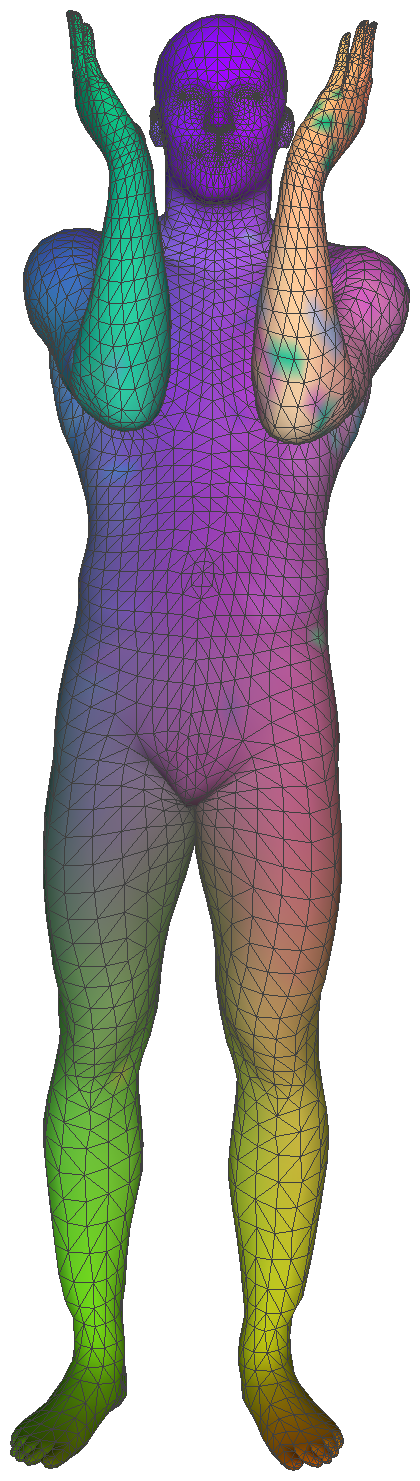} &
	\includegraphics[scale=0.061]{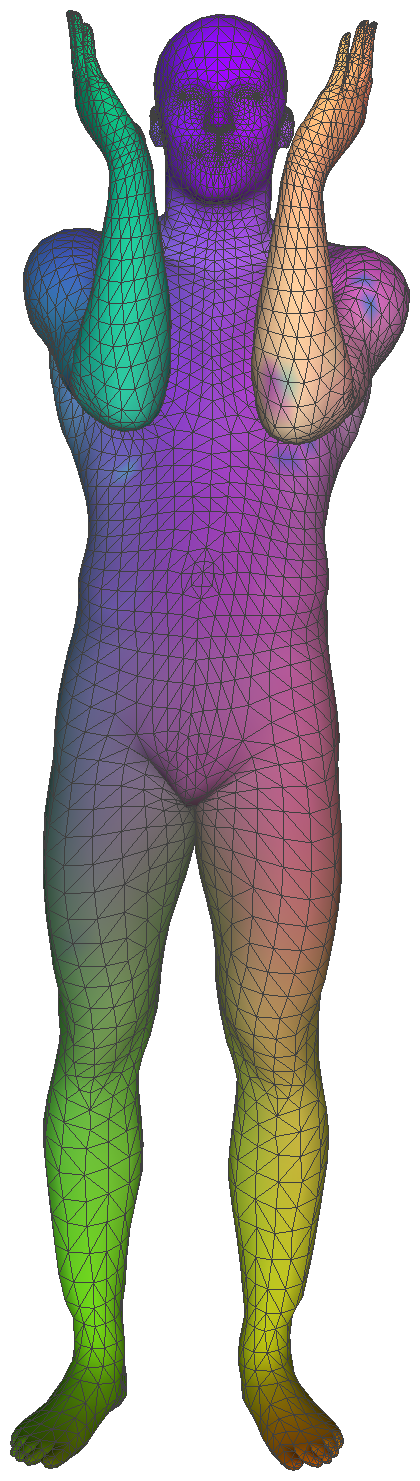} &
	\includegraphics[scale=0.054]{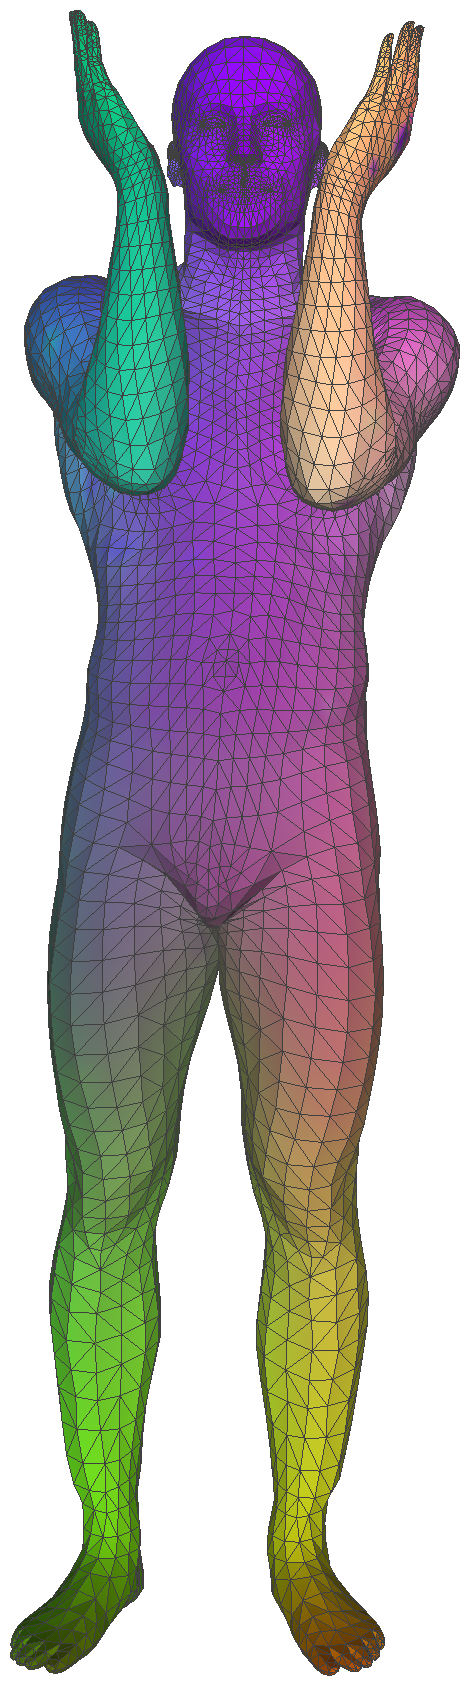} &
	\includegraphics[scale=0.054]{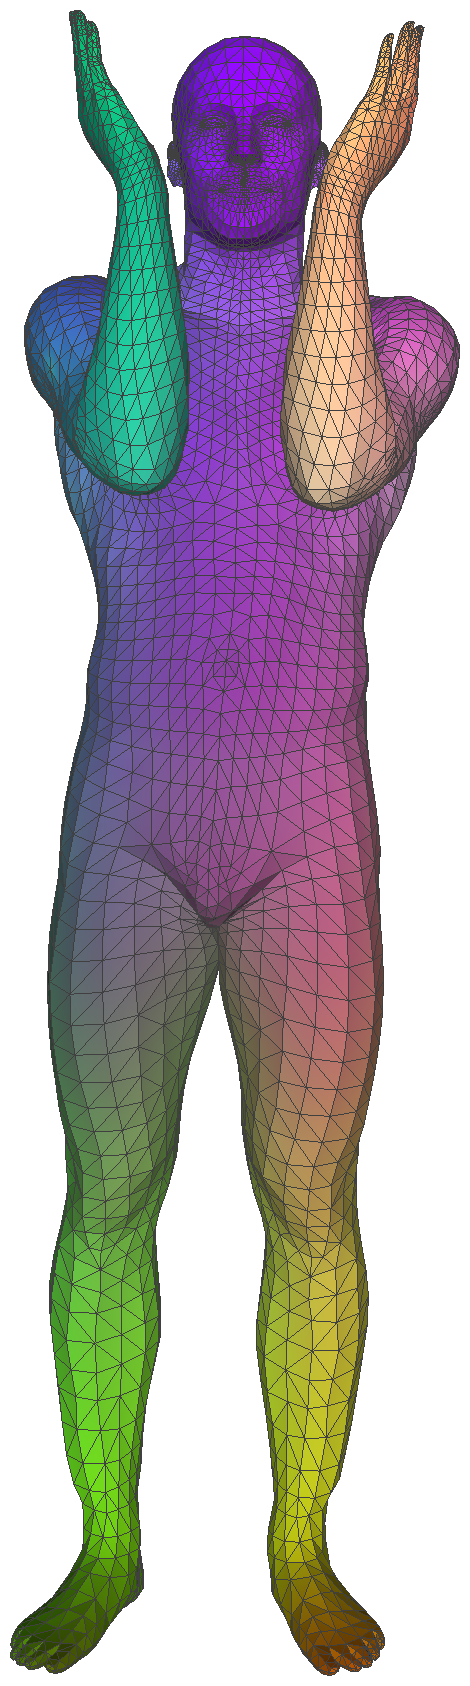} &
	\includegraphics[scale=0.054]{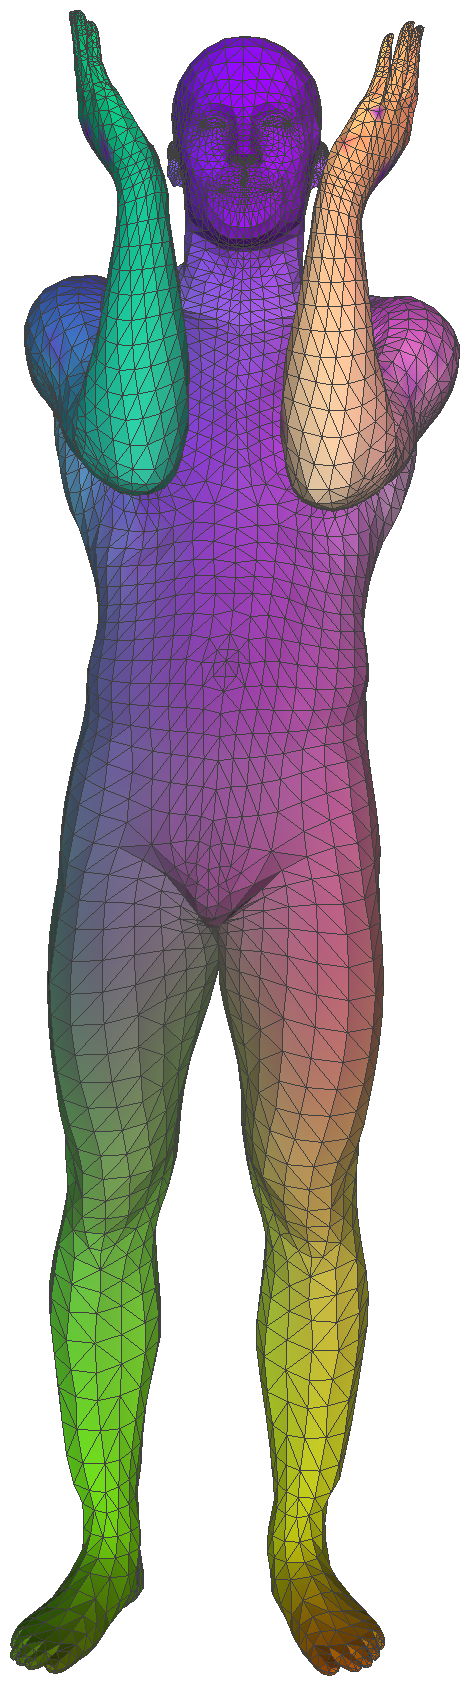}
	\\
	 &
	\includegraphics[height=40px]{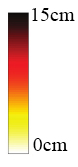} &
	\includegraphics[scale=0.054]{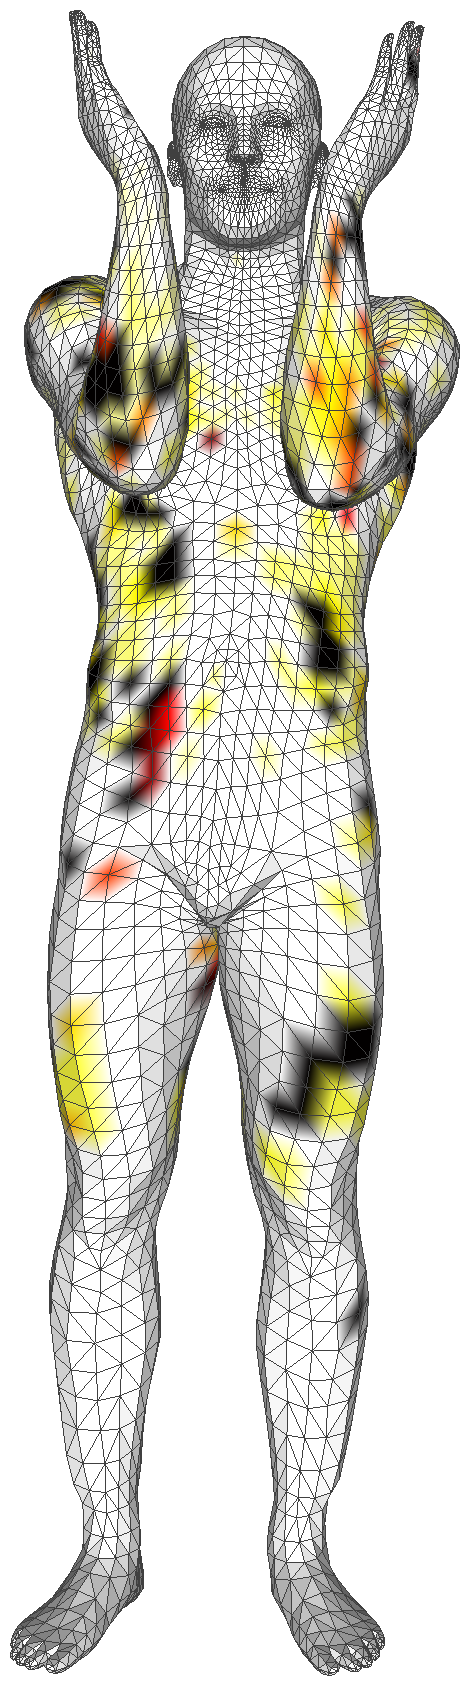} &
	\includegraphics[scale=0.054]{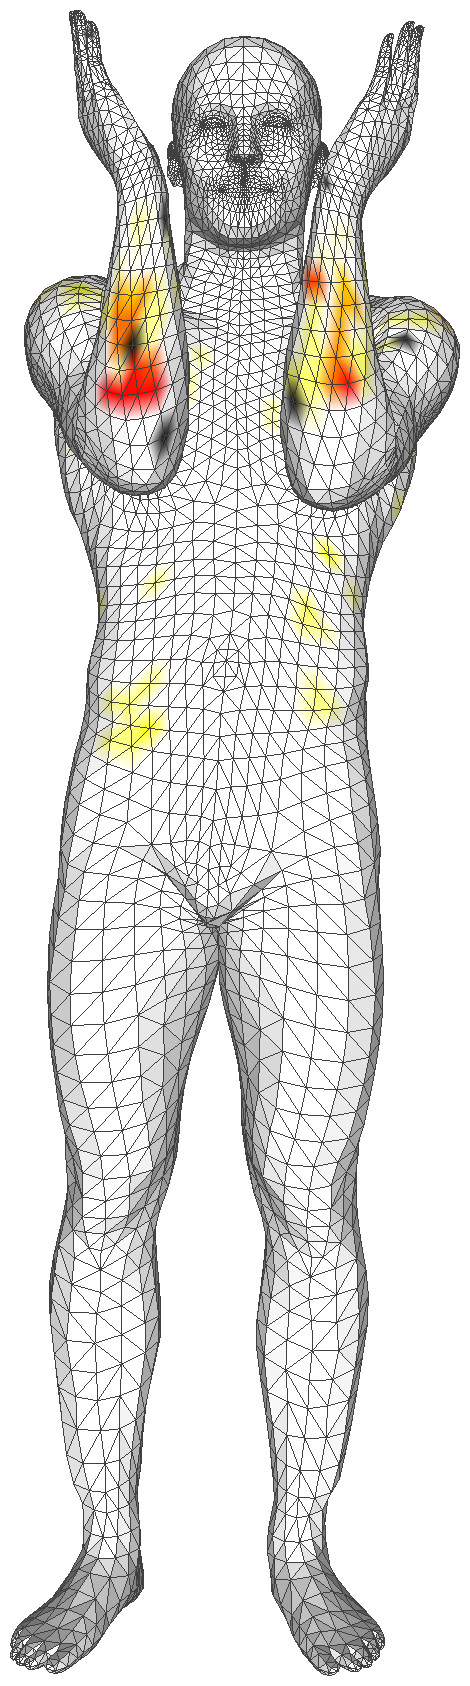} &
	\includegraphics[scale=0.059]{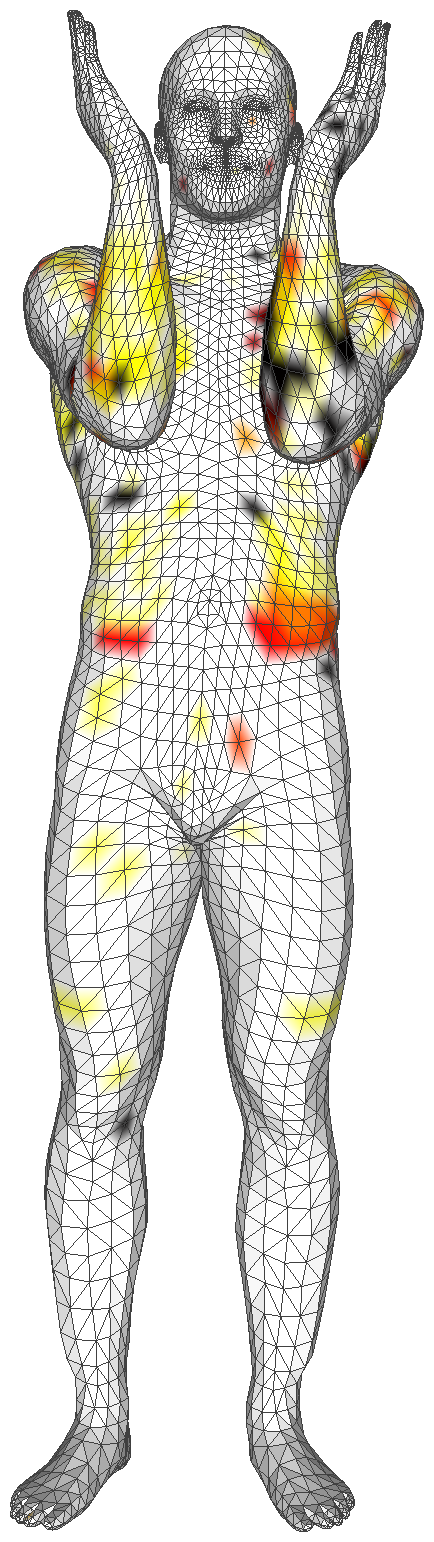} &
	\includegraphics[scale=0.059]{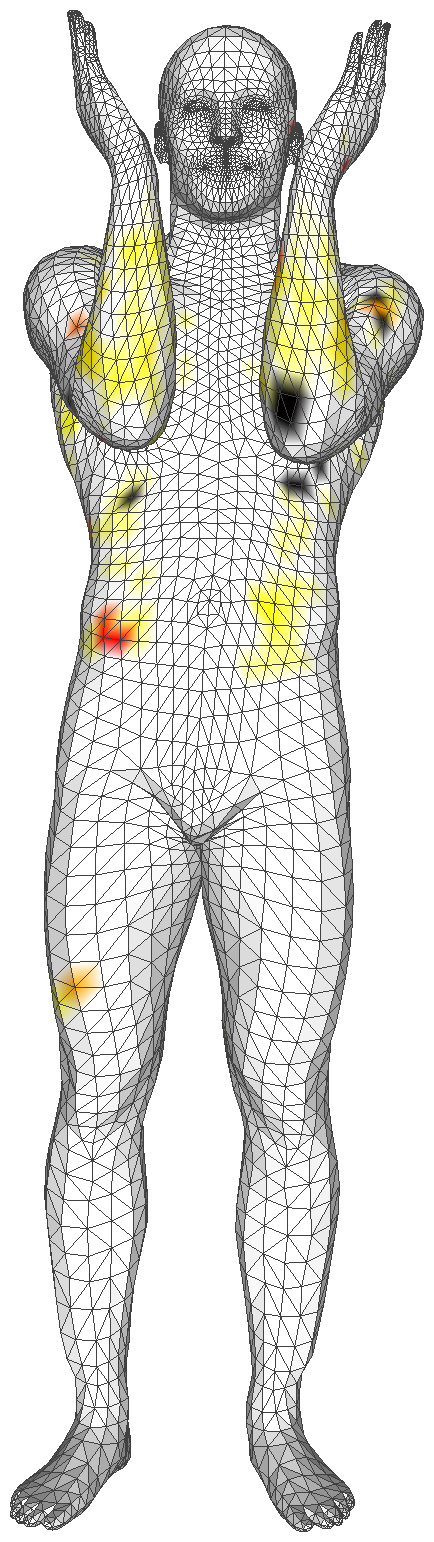} &
	\includegraphics[scale=0.054]{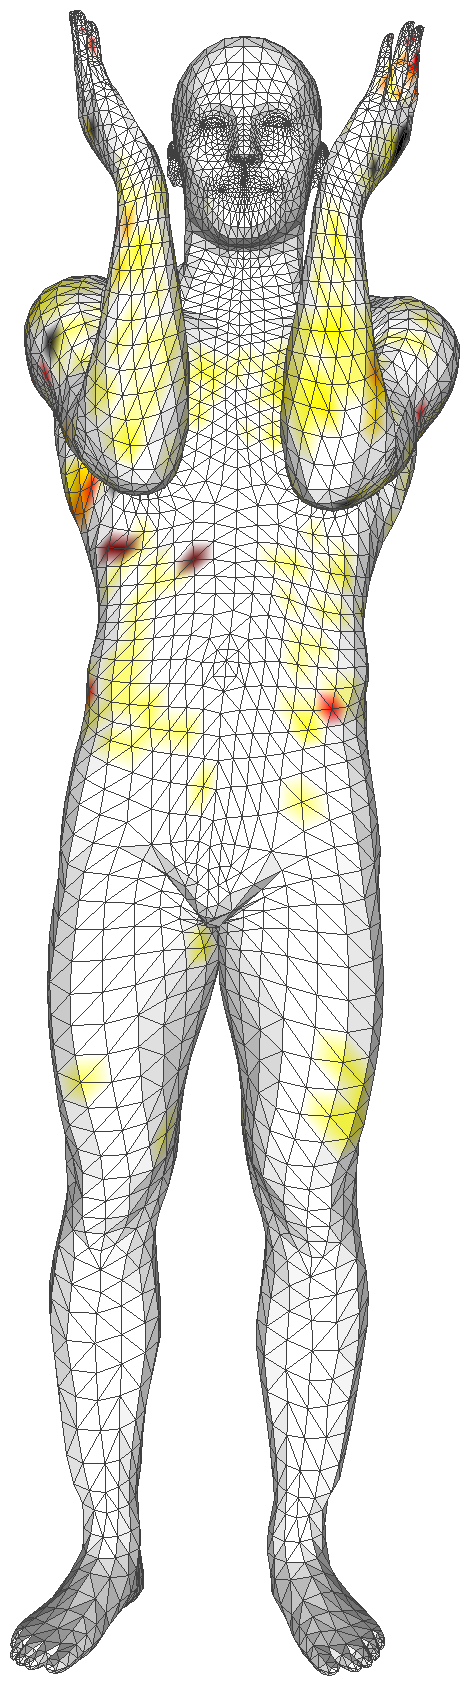} &
	\includegraphics[scale=0.054]{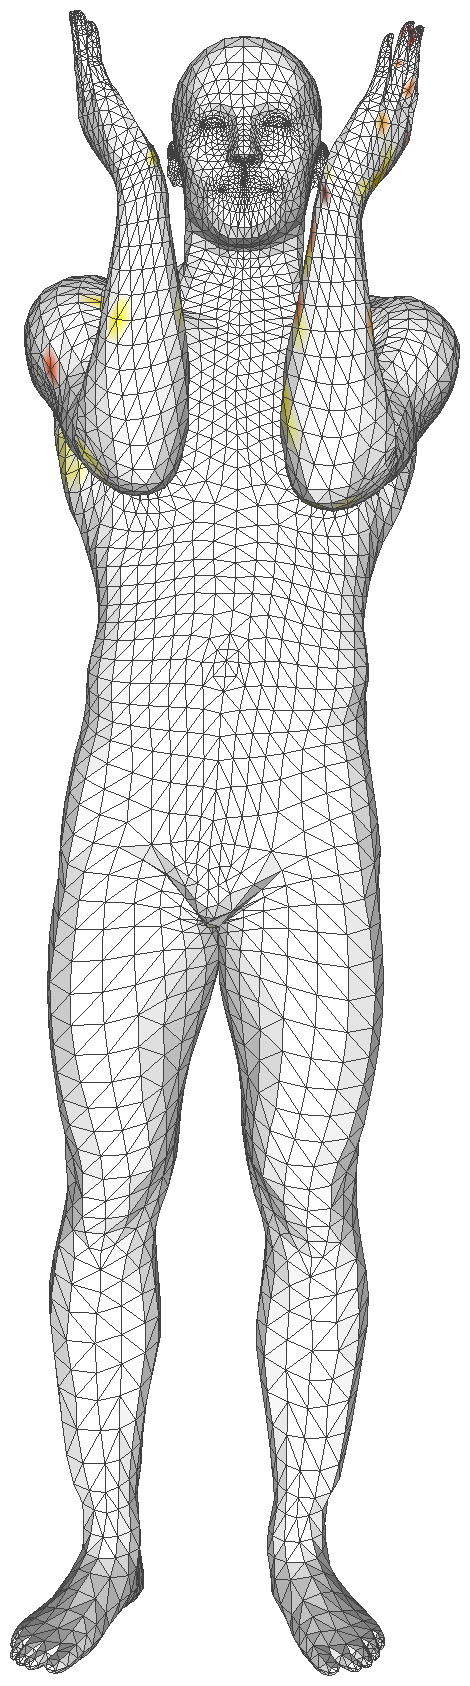} &
	\includegraphics[scale=0.054]{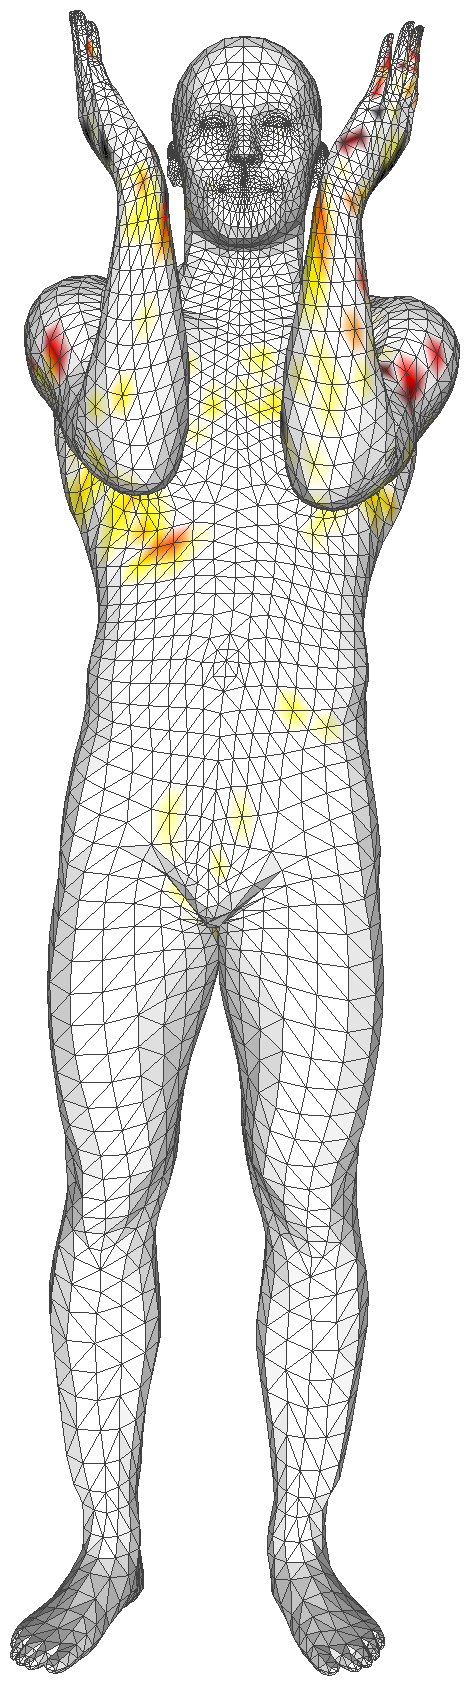}
	\\ 
	\midrule
	{\rotatebox{90}{\tiny{$50\%$}}} &
	\includegraphics[scale=0.042]{remeshed_faust_plots/faust_ref}  &
	\includegraphics[scale=0.054]{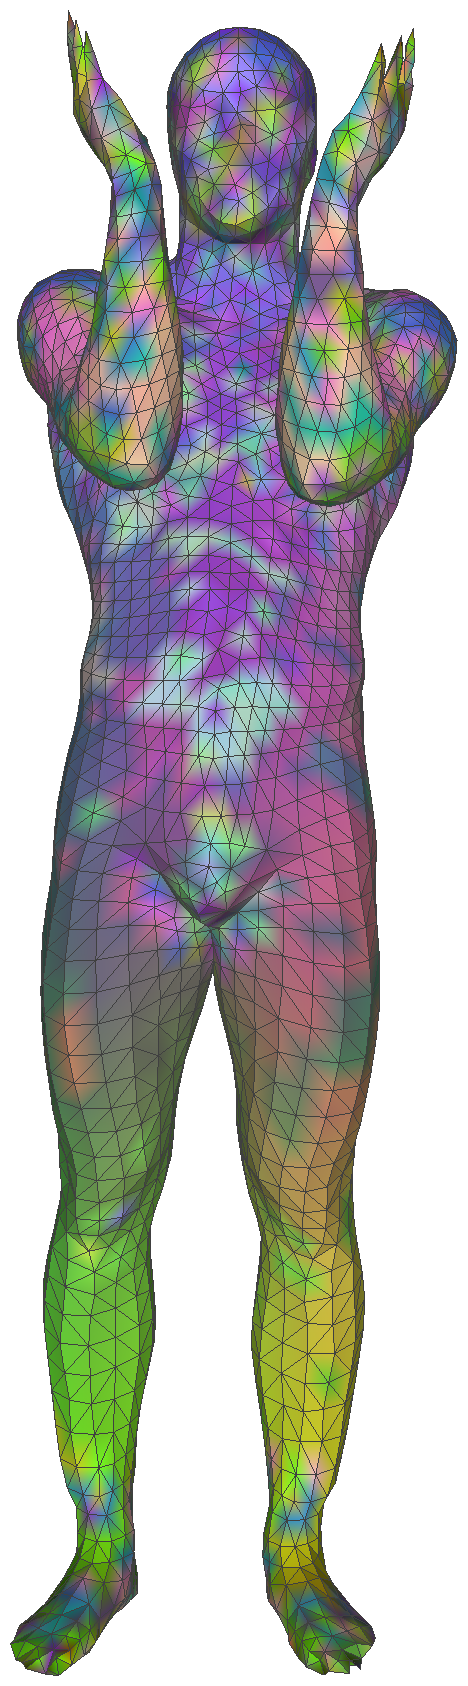} &
	\includegraphics[scale=0.054]{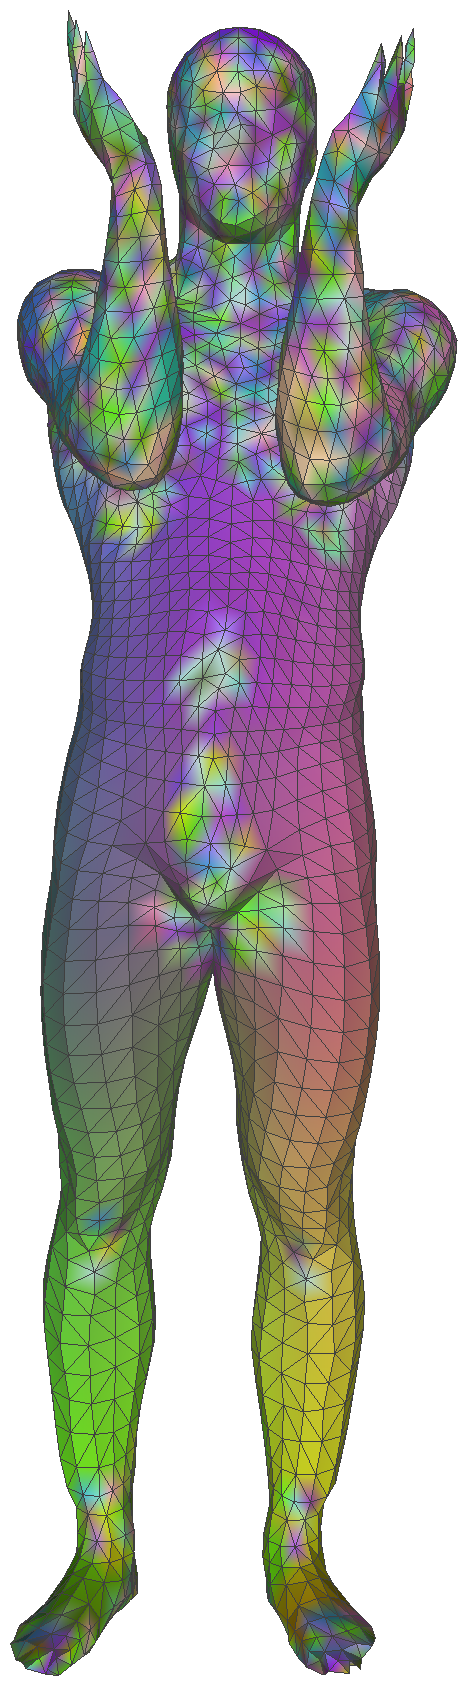} &
	\includegraphics[scale=0.061]{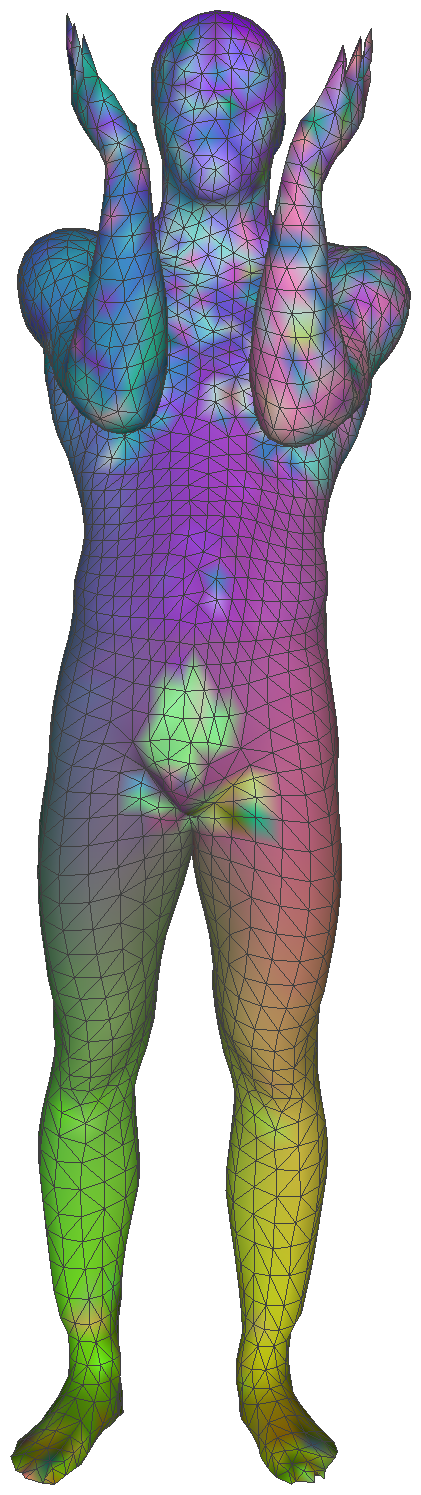} &
	\includegraphics[scale=0.061]{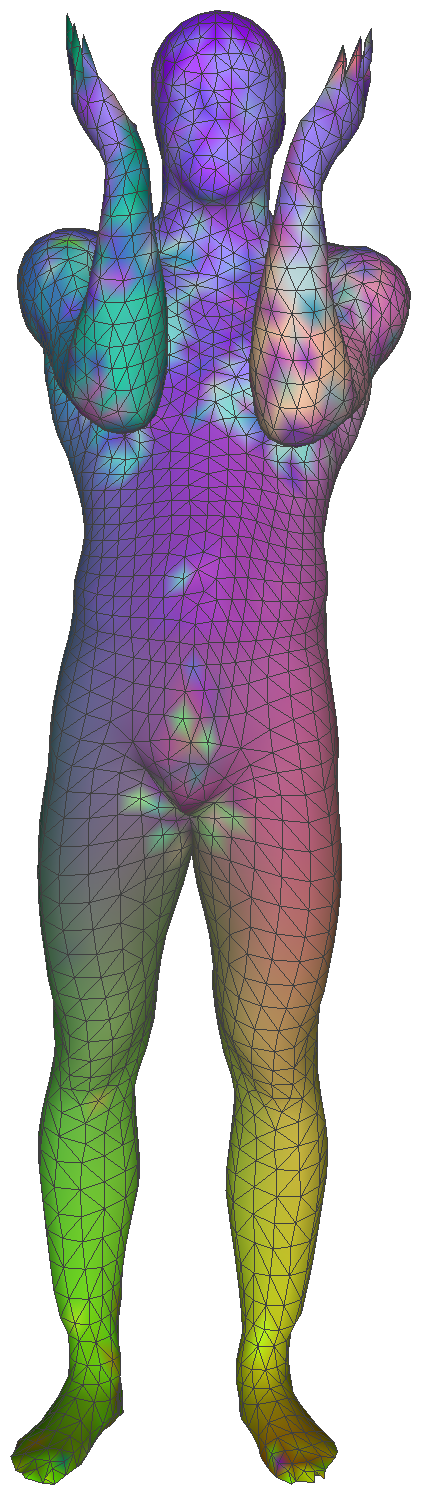} &
	\includegraphics[scale=0.054]{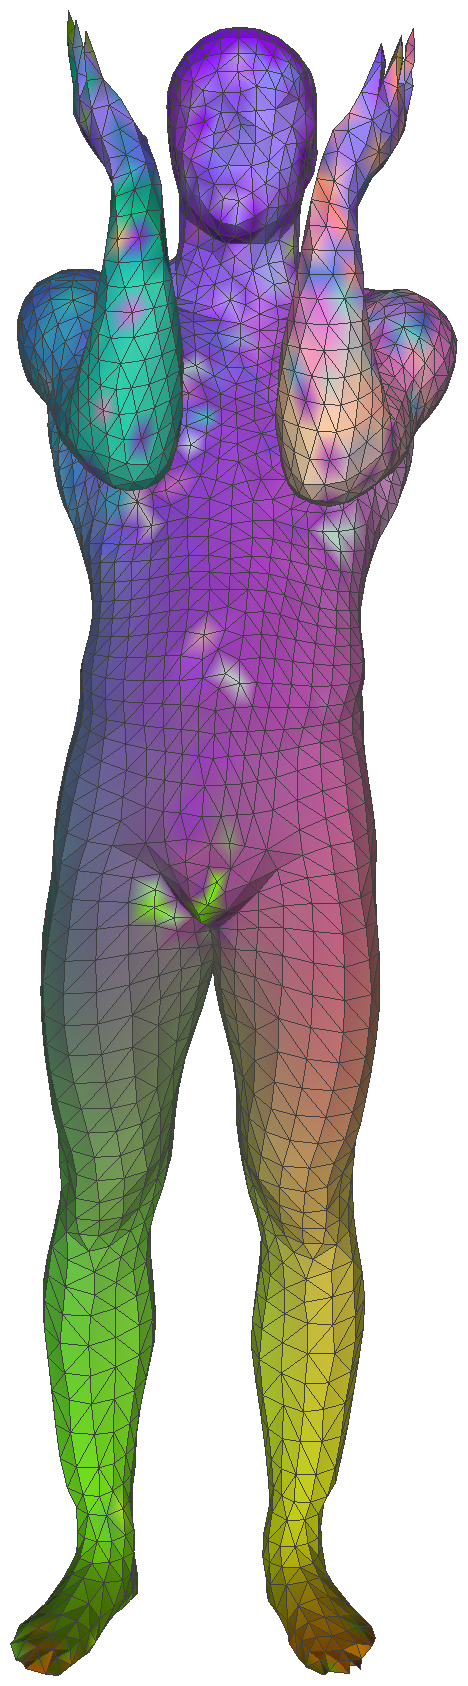} &
	\includegraphics[scale=0.054]{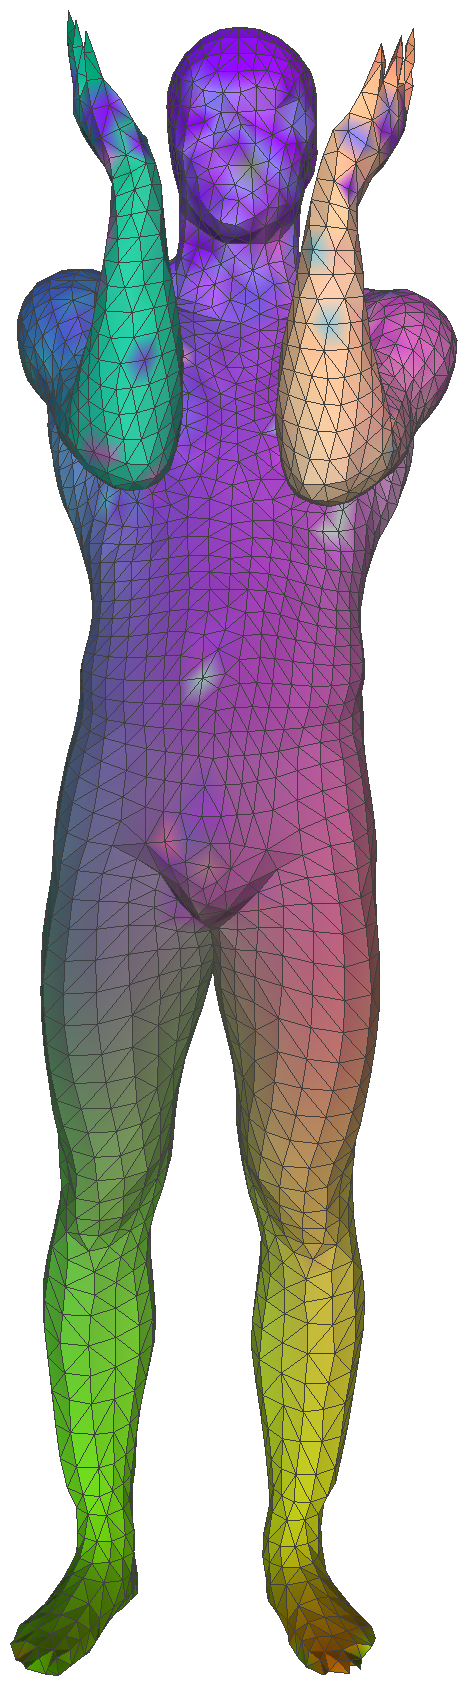} &
	\includegraphics[scale=0.054]{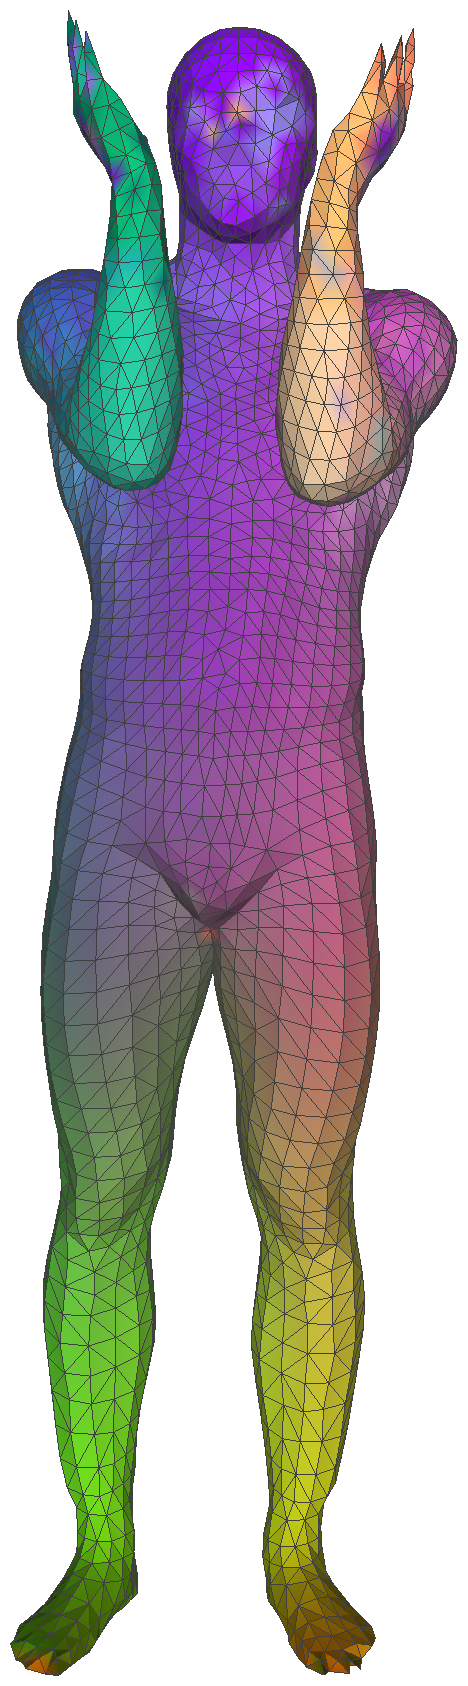}
	\\
	 &
	 \includegraphics[height=40px]{figures/errors_colormap} &
	 \includegraphics[scale=0.054]{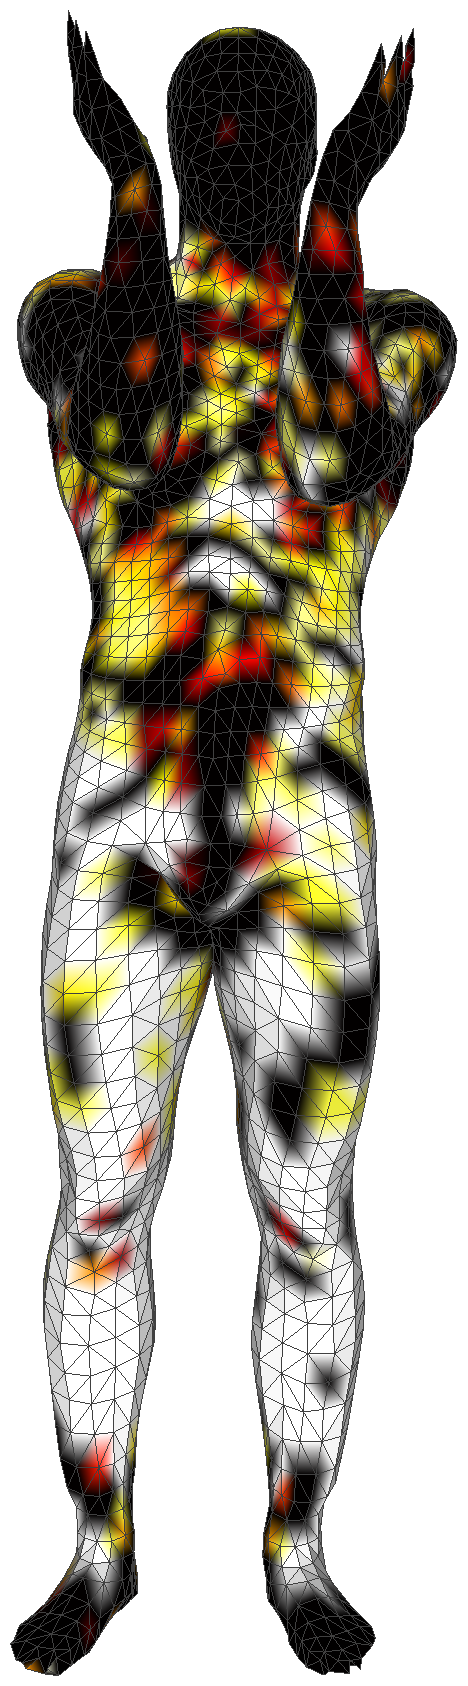} &
	 \includegraphics[scale=0.054]{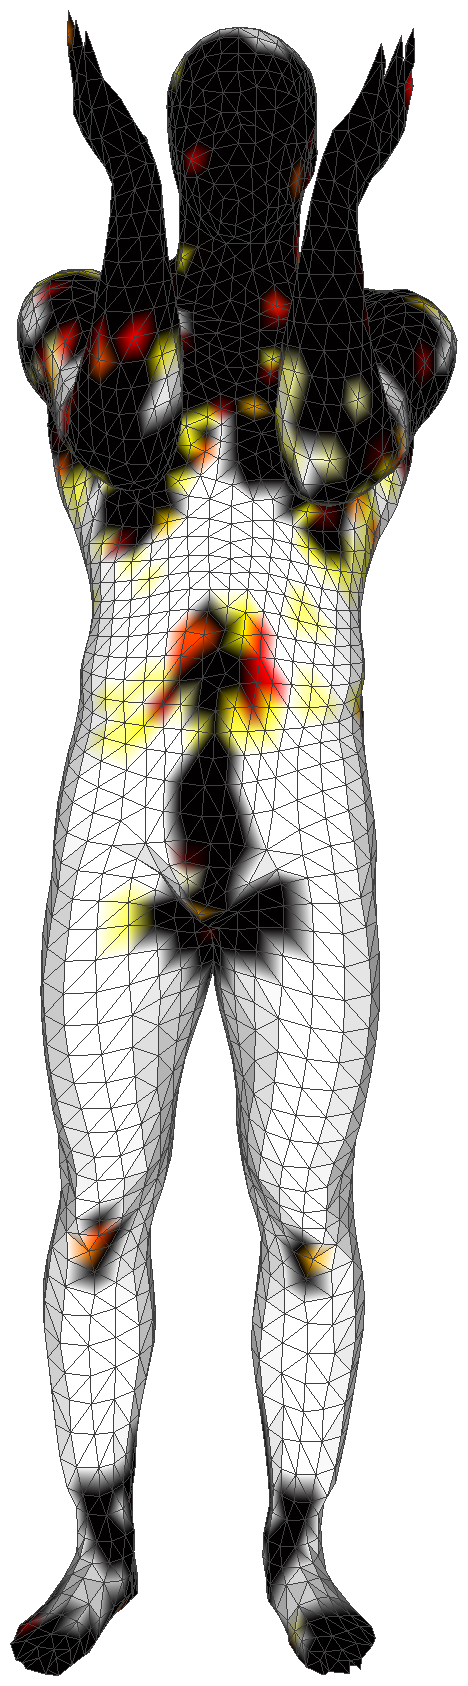} &
	\includegraphics[scale=0.059]{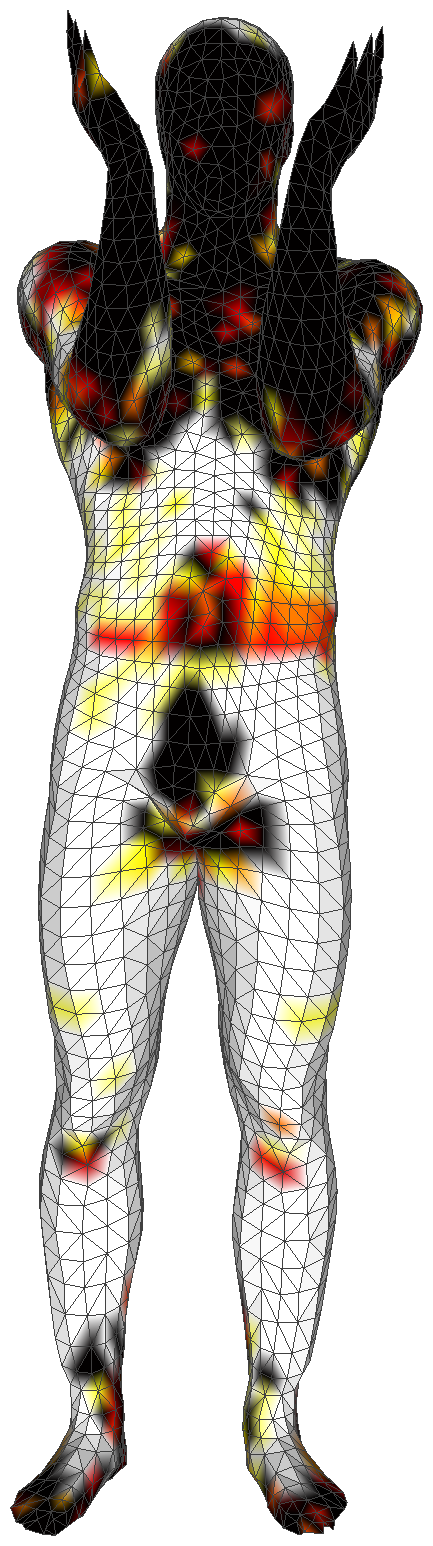} &
	\includegraphics[scale=0.059]{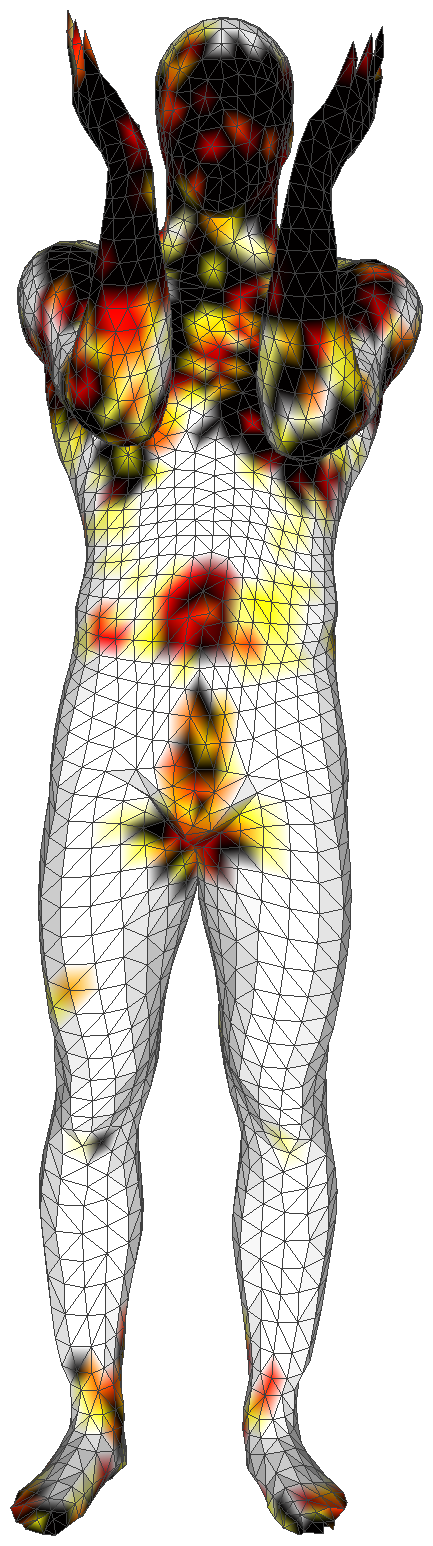} &
	\includegraphics[scale=0.054]{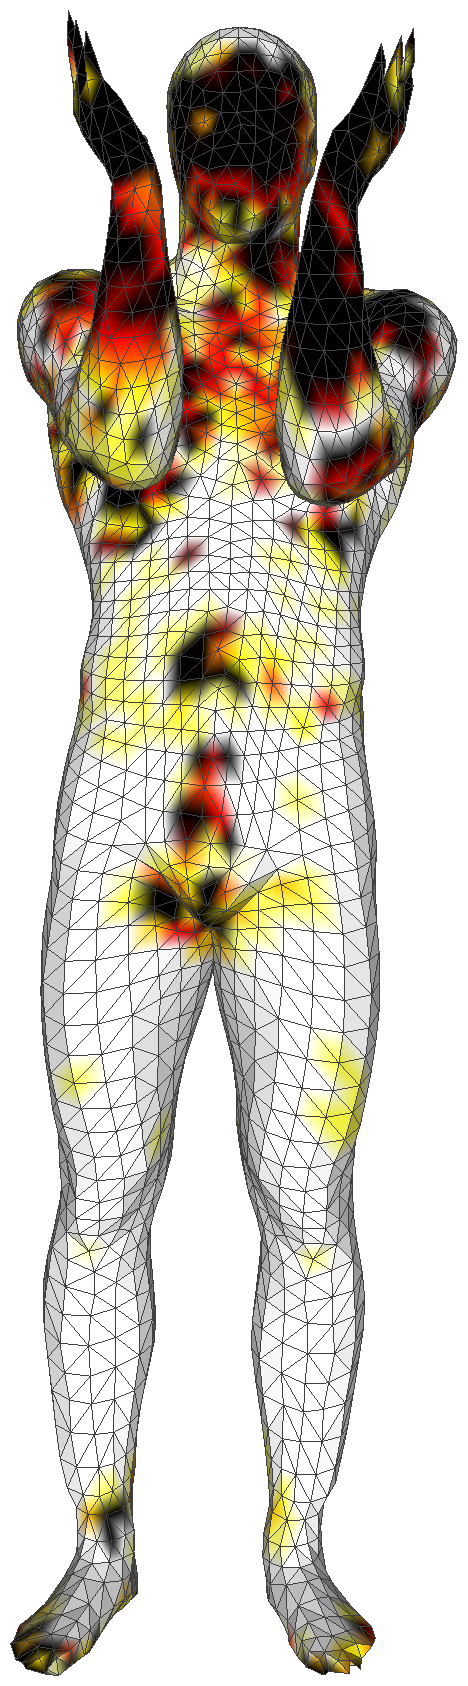} &
	\includegraphics[scale=0.054]{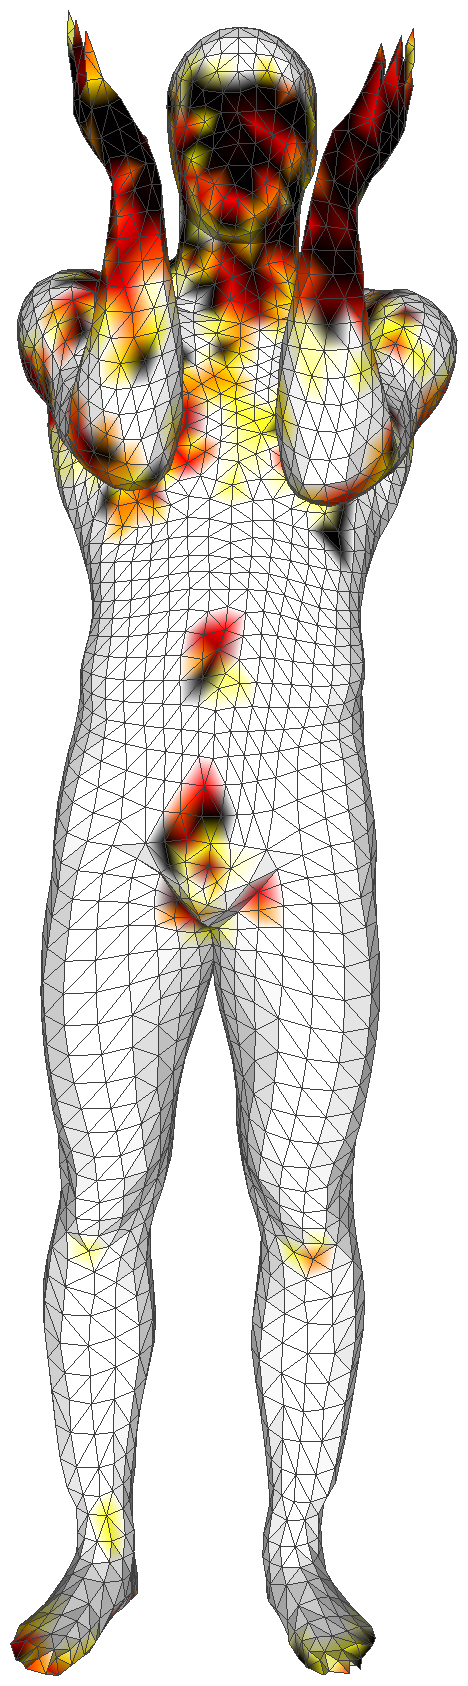} &
	\includegraphics[scale=0.054]{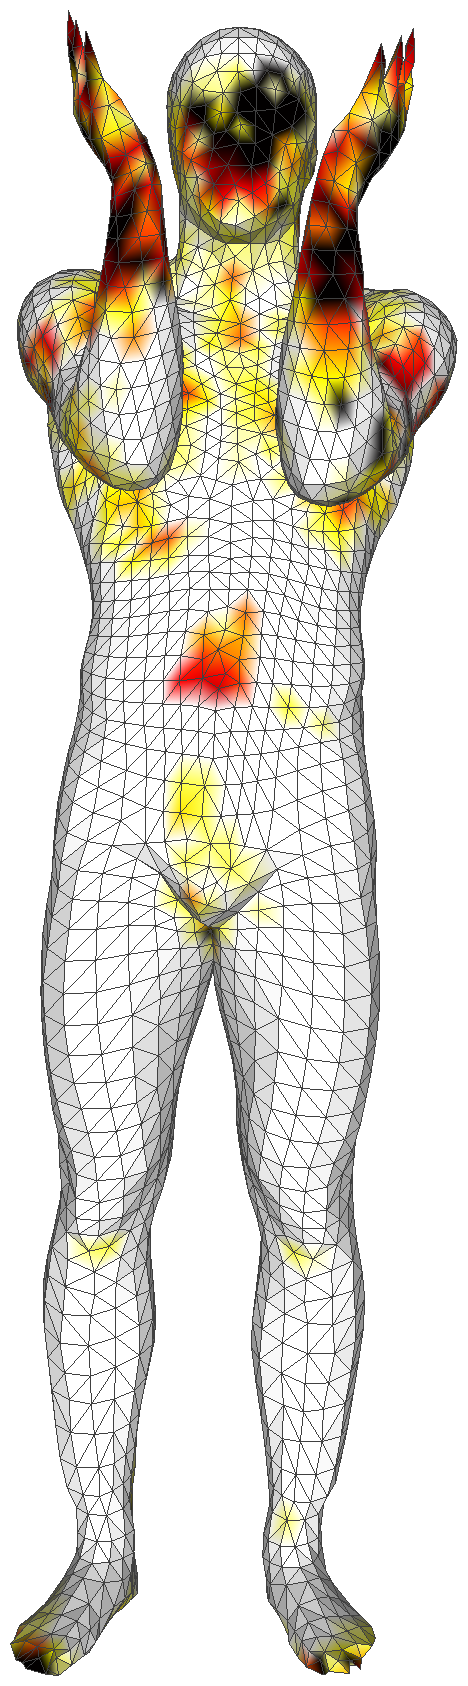}
	\\
	 & \textbf{Faust-Synthetic} & \textbf{MoNet} & \textbf{SplineCNN} & \textbf{FeaStNet} & \multicolumn{2}{c|}{\textbf{FeaStNet--Dual}} & \multicolumn{2}{c}{\textbf{DualConvMax}}
	\\
	 & \textbf{Reference} & \scriptsize{(SHOT)} & \scriptsize{(XYZ)} & \scriptsize{(XYZ)} & \scriptsize{(XYZ)} & \scriptsize{(XYZ+Normal)} & \scriptsize{(XYZ)} & \scriptsize{(XYZ+Normal)}
	\\
	\end{tabular}
}
\caption{Visualizations of texture transfer and geodesic correspondence errors for a full resolution Faust-Synthetic test mesh (top two rows), and the same mesh decimated by 50\% (bottom two rows) of the Faust-Decimated dataset. Models are trained on the full resolution Faust-Synthetic meshes.
}
\label{fig:faust_decimated_errors}
\end{figure*}
